# Supplementary material for: Microscopic view on the ultrafast photoluminescence from photo-excited graphene
Source: arXiv:1411.0531 source file (2014-11-03)
Supplement: Supplementary file 1 [file supplementary.pdf]

# Supplementary information for: Microscopic view on the ultrafast photoluminescence from photo-excited graphene

Torben Winzer[1,2], Richard Ciesielski[3], Matthias Handloser[3],
Alberto Comin[3], Achim Hartschuh[3], and Ermin Malić[1]
[1]*Institut für Theoretische Physik, Technische Universität Berlin, Hardenbergstr. 36, 10623 Berlin, Germany*
[2]*Department of Materials Science and Engineering, Yonsei University, Seoul 120-749, Korea and*
[3]*Department Chemie und CeNS, Ludwig Maximilians Universität München, Butenandtstr. 5-13, 81377 Munich, Germany**

## I. EXPERIMENTAL SETUP

Emission spectra were recorded for few layer graphene using a scanning confocal microscope with NA = 1.3. The spectral and temporal characteristics of the broadband laser excitation pulse provided by a Ti:Sa oscillator were controlled using a 4f pulse shaper (Fig. S1(a)).

The Ti:Sa oscillator has a controllable bandwidth of 750 - 850 nm resulting in pulses of a length of around 15 fs. The key element of the pulse shaper is a liquid crystal dual line array for spectral amplitude and phase shaping. The optical signal is transmitted by the beam splitter and detected either by an avalanche photodiode (APD) after spectral filtering using a bandpass filter or by a spectrometer equipped with a silicon-based CCD camera and an InGaAs linear array. With the confocal microscope it is possible to record scan images and to address selected sample areas.

Optical components in the excitation beam path such as lenses, dielectric filters and especially the microscope objective cause a strong temporal broadening of the laser pulse. With the pulse shaper these phase distortions can be compensated by applying the inverse, resulting in a flat phase (bandwidth limited) pulse in the focus. Using the second harmonic generation (SHG) of a reference material ($Fe(IO_3)_3$ in our case) we determined the phase distortions in every used measurement configuration by the well known method of multiphoton intrapulse interference phase scans (MIIPS, see[1,2]). The most relevant part of the phase is the group delay dispersion (GDD) which we can measure and compensate with an accuracy of max. $10 fs^2$ over the full spectrum. After the pulse has been compressed in the focus, the SHG is used to additionally verify the pulse length by interferometric autocorrelation scans, showing a very good agreement with the theoretically expected pattern based on the recorded laser spectrum (Fig. S1(b)).

For the experiment, the laser excitation energies and the detection ranges were selected to exclude signal contributions from four-wave mixing[3] such that $\omega_{detected} \neq \omega_3 = 2\omega_1 - \omega_2$ for all $\omega_{1,2}$ within the excitation range.

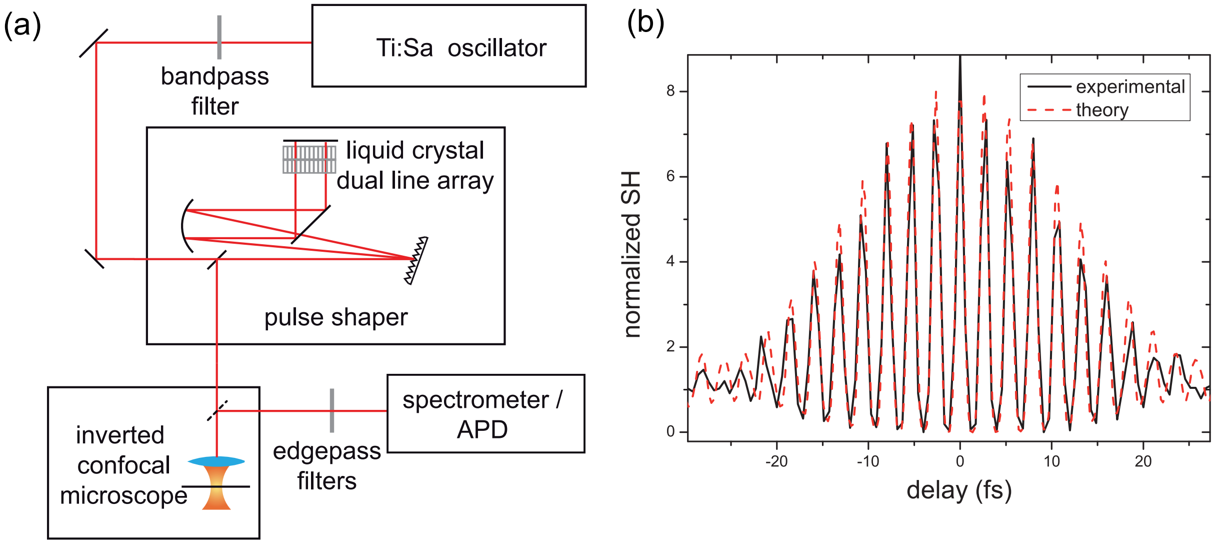


FIG. S1: (a) Simplified schematic of the setup. (b) Exemplary second harmonic (SH) auto-correlation scan using the shaper after compression of the full bandwidth pulse on $Fe(IO_3)_3$. The theoretical curve was calculated from the recorded laser spectrum and agrees very well with the measured data, which has been divided by the value at full separation (500 fs). The good agreement is a verification of the successful intra-focus pulse compression.

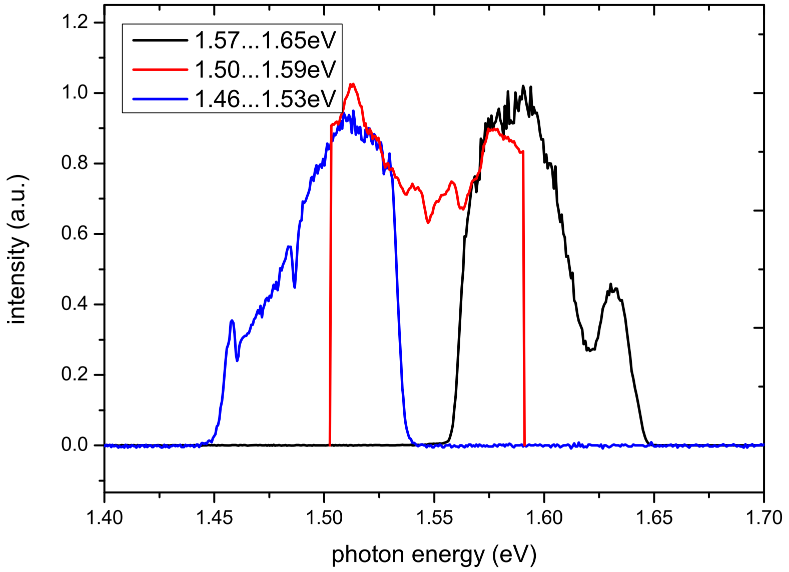


FIG. S2: Laser spectra used to record the emission spectra in Fig. 5 of the main manuscript.

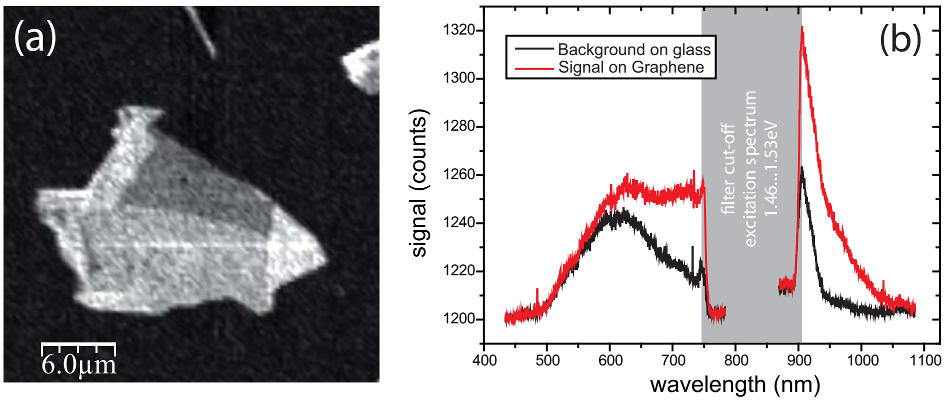


FIG. S3: (a) Typical confocal PL scan of a few layer flake of exfoliated graphene on glass detecting the emission between 950 and 1020 nm. The PL image has been recorded using the full excitation spectrum (750 - 850 nm). (b) Raw spectral data taken on the graphene flake (red curve) and directly next to it representing the signal background (black curve). Spectra taken on glass were used for background correction of the emission spectra shown in Fig. 5 in the main manuscript.

The three laser spectra used in Fig. 5 of the main manuscript are shown in Fig. S2. The laser spectra were cut from the full available bandwidth using a combination of steep edge or bandpass filters. For each laser spectrum we recompressed the intra-focus pulses as described above.

## II. BACKGROUND CORRECTION

All emission spectra were corrected for a weak background signal resulting from residual laser scattered light, the response of the glass substrate and of the microscope objective. The background signal was recorded on the glass substrate next to the graphene flakes (Fig. S3). The sensitivity and transmission of the detection setup (lenses, gratings, detectors) was separately measured by a calibrated black body radiation source. All spectra were corrected for the spectral characteristics of the setup.

## III. POWER DEPENDENCE OF EMISSION SPECTRA

Fig. S4 presents the power dependence of the emission spectrum in the red spectral range between 1.1 and 1.2 eV for which the largest variations are predicted by our theoretical modelling. For the high power regime the signals increases slightly towards lower energies while for the low power regime the signal clearly drops for lower energies. This is in agrement with the spectra presented in Fig. 4(a) and (b) in the main manuscript.

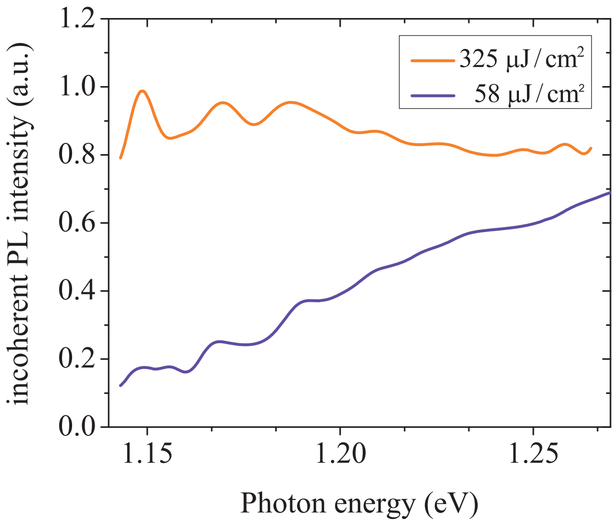


FIG. S4: Emission spectra recorded in the near infrared for two different excitation fluences. For the high power regime the signals is slightly increasing towards lower energies and for the low power regime the signal clearly drops for lower energies. The detection range was chosen such that the fluence dependence is most pronounced with a strongly increased contribution from the incoherent PL. (The small spectral modulation is due to the filter transmission.)

---


* ermin.malic@tu-berlin.de


[1] B. Xu, Y. Coello, V. V. Lozovoy, D. A.. Harris, and M. Dantus, Opt. Express **14**, 10939 (2006).
[2] A. Comin, R. Ciesielski, G. Piredda, K. Donkers, and A. Hartschuh, J. Opt. Soc. Am. B **5**, 1118 (2014).
[3] E. Hendry, P. J. Hale, J. Moger, A. K. Savchenko, and S. A. Mikhailov, Phys. Rev. Lett. **105**, 097401 (2010).
